# Supplementary material for: Grid Tariffs Based on Capacity Subscription: Multi Year Analysis on Metered Consumer Data
Source: arXiv:2111.06253 source file (2021-11-05)
Supplement: Supplementary file 1 [file Appendix.tex]

\appendix
\appendixpage
\addappheadtotoc

\begin{appendices} \label{Appendix}

\end{appendices}
